# Supplementary material for: Neutrino Physics with JUNO
Source: arXiv:1507.05613 source file (2015-10-18)
Supplement: Supplementary file 1 [file ThisSection.tex]

\documentclass[dvipdfm,11pt,a4paper]{article}
\usepackage[dvips]{graphicx,color}
\usepackage[bookmarks]{hyperref}
\usepackage{url}
\usepackage{amssymb}
\usepackage[centertags]{amsmath}

\makeatletter
\renewcommand{\thefigure}{\ifnum \c@section>\z@ \thesection-\fi \@arabic\c@figure}
\renewcommand{\thetable}{\ifnum \c@section>\z@ \thesection-\fi \@arabic\c@table}
\@addtoreset{equation}{section}
\makeatother

\oddsidemargin 0.in
\textheight 9.0in
\textwidth  6.5in
\parindent=20pt
\baselineskip 12pt

\begin{document}
\input{main.tex}

\end{document}
